# Supplementary material for: Simultaneously enhancing brightness and purity of WSe$_2$ single photon emitter using high-aspect-ratio nanopillar array on metal
Source: arXiv:2409.15819 source file (2024-09-24)
Supplement: Supplementary file 1 [file si.pdf]

Supporting Information for:

# Simultaneously enhancing brightness and purity of $WSe_2$ single photon emitter using high-aspect-ratio nanopillar array on metal

Mayank Chhaperwal[1], Himanshu Madhukar Tongale[1], Patrick Hays[2], Kenji Watanabe[3], Takashi Taniguchi[4], Seth Ariel Tongay[2] and Kausik Majumdar[1*]

[1]Department of Electrical Communication Engineering,
Indian Institute of Science, Bangalore 560012, India

[2]Materials Science and Engineering, School for Engineering of Matter, Transport and Energy,
Arizona State University, Tempe, Arizona 85287, USA

[3]Research Center for Electronic and Optical Materials,
National Institute for Materials Science, 1-1 Namiki, Tsukuba 305-044, Japan

[4]Research Center for Materials Nanoarchitectonics,
National Institute for Materials Science, 1-1 Namiki, Tsukuba 305-044, Japan

[*]Corresponding author, email: kausikm@iisc.ac.in

# Supporting Information 1: Methods

## SPE fabrication

20/40 nm thick Ti/Au film is sputter coated on Si substrate covered with 285 nm thick thermally grown $SiO_2$. A negative tone resist (ma-N-2403 from micro resist technology) is spin-coated on the substrate at 3000 rpm for 30 seconds to get a uniform layer of 300 nm thickness. The substrate is heated at 90°C for 2 minutes to cure the resist. A pattern with solid circles is defined on this substrate via electron beam lithography using an accelerating voltage of 30 kV and an aperture of 10 $\mu$m. The diameter of the circles is kept at 150 nm, and an array is patterned with a spacing of 5 $\mu$m. The electron beam hardens the negative resist in the location of the patterned circles. The substrate is then developed with AZ-726 MIF developer to remove the unwanted resist. The substrate is hard-baked at 150°C for 15 minutes to increase the mechanical strength of the nanopillars for transferring layers on top of them.

$WSe_2$ is exfoliated on a polydimethylsiloxane (PDMS) sheet and an appropriate monolayer flake is identified. We then use micro-manipulators to transfer this flake onto the patterned nanopillars. A few-layer thick hBN flake is then transferred on top using the same method. The entire structure is then annealed in vacuum ($10^{-6}$ mbar) at 150°C for 3 hours.

## SPE Characterization

**Photoluminescence:** All PL measurements are carried out at 5 K temperature with a ×50 objective (numerical aperture of 0.5). The excitation source used is a 532 nm laser operated in CW mode unless otherwise stated. The spot size for the laser is ∼1.5 $\mu$m. PL spectra are recorded with a spectrometer consisting of a grating with 1800 lines per mm and CCD. For the photoluminescence excitation (PLE) measurement, a supercontinuum source is used with a tunable narrow-band filter to vary the excitation wavelength.

**TRPL:** TRPL measurement is performed at 5 K with a 705 nm laser head (from PicoQuant) operated through a laser drive (PDL-800D) in pulsed mode with a 10 MHz repetition rate. Output from the SPE is guided to a single photon detector (SPD-050-CTC from Micro Photon Devices) via a combination of a long pass filter (cut in wavelength of 750 nm) and a tunable monochromator (Edmund optics) with a resolution of 0.5 nm. Time correlations are performed

by a time-correlated single photon counting (TCSPC) system (PicoHarp 300 from PicoQuant). The IRF of the entire TRPL setup is ∼60 ps. Data from the measurement is fitted with an exponential decay convoluted with a Gaussian rise function given by $F(t) = \frac{1}{\sigma\sqrt{2\pi}}e^{\frac{-(t-\tau_f)^2}{2\sigma^2}}$ where $\tau_f$ is the formation time measured from the laser excitation time.

**Second-order correlation:** second-order correlation measurements are performed with a CW excitation at 5 K. PL emission from the device is passed through a long pass filter (cut in wavelength of 750 nm) to remove the scattered laser component and then through a tunable monochromator (Edmund optics) with a resolution of 0.5 nm to select the SPE emission wavelength. The photons then go through a beamsplitter (from Thorlabs) and two single-photon detectors [from Excelitas] arranged in an HBT setup. The detectors are connected to the TCSPC system (PicoHarp 300 from PicoQuant), which generates a histogram of coincidence counts between the two outputs as a function of delay ($\tau$) between them through QuCoa software (from PicoQuant). The plot is then normalized with respect to that of a coherence source such that the value of $g^{(2)}(\tau)$ is 1 for $\tau$ much larger than the lifetime of the emitter. Measured coincidences are normalized with that from a coherent source and are plotted in **??**f with varying delay ($\tau$) between the two detectors. The timing jitter (250 ps) of the SPADs, being comparable to $\tau_d$, modifies the slope and the value of the anti-bunching dip. The $g^{(2)}(\tau)$ curve is then deconvoluted from the Gaussian instrument response function (IRF) of the HBT setup arising from the finite timing jitter of the detectors (250 ps each) and the finite bin size used in the QuCoa software for calculating the correlation (50 ps for the measurement at higher emission rate and 100 ps for the measurement at lower emission rate).

## Supporting Information 2: Line cut from the PL map

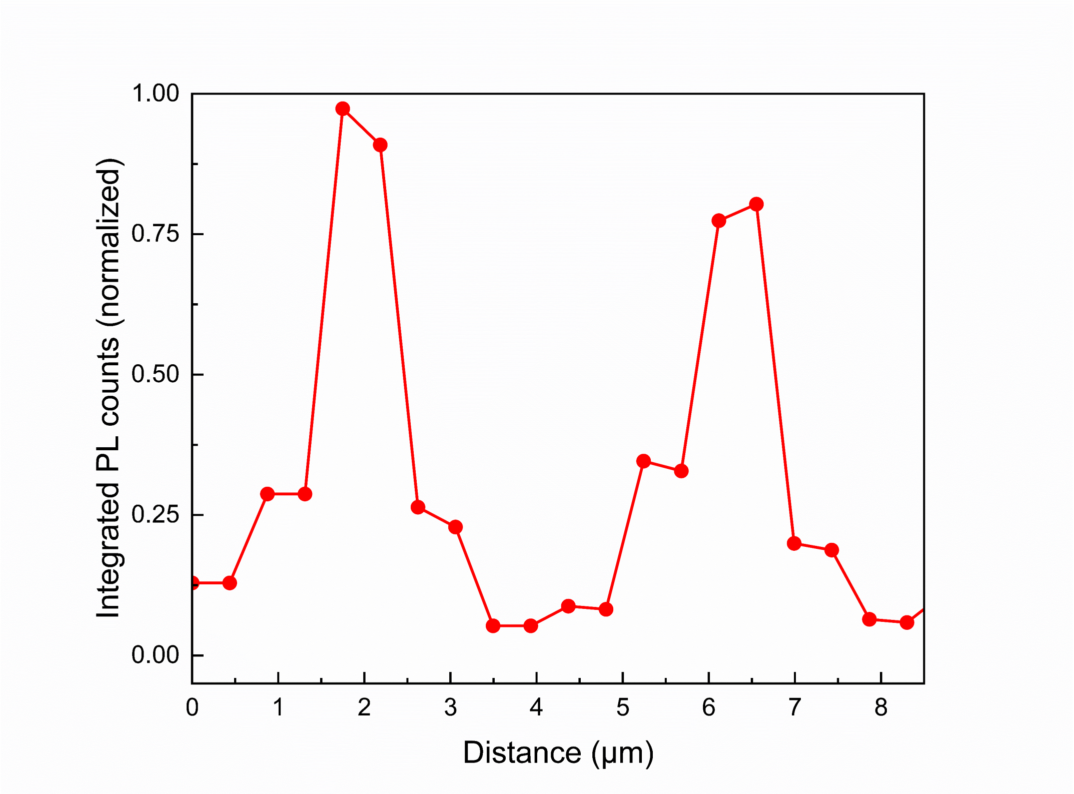


Supporting Figure 1: **Line cut from the PL map.** Integrated exciton emission taken from two of the brightest nanopillars from the PL map show the suppression of emissions from the flat regions compared to that from the nanopillars.

## Supporting Information 3: Measurement of count rate: SPAD count rate versus pure SPE count rate

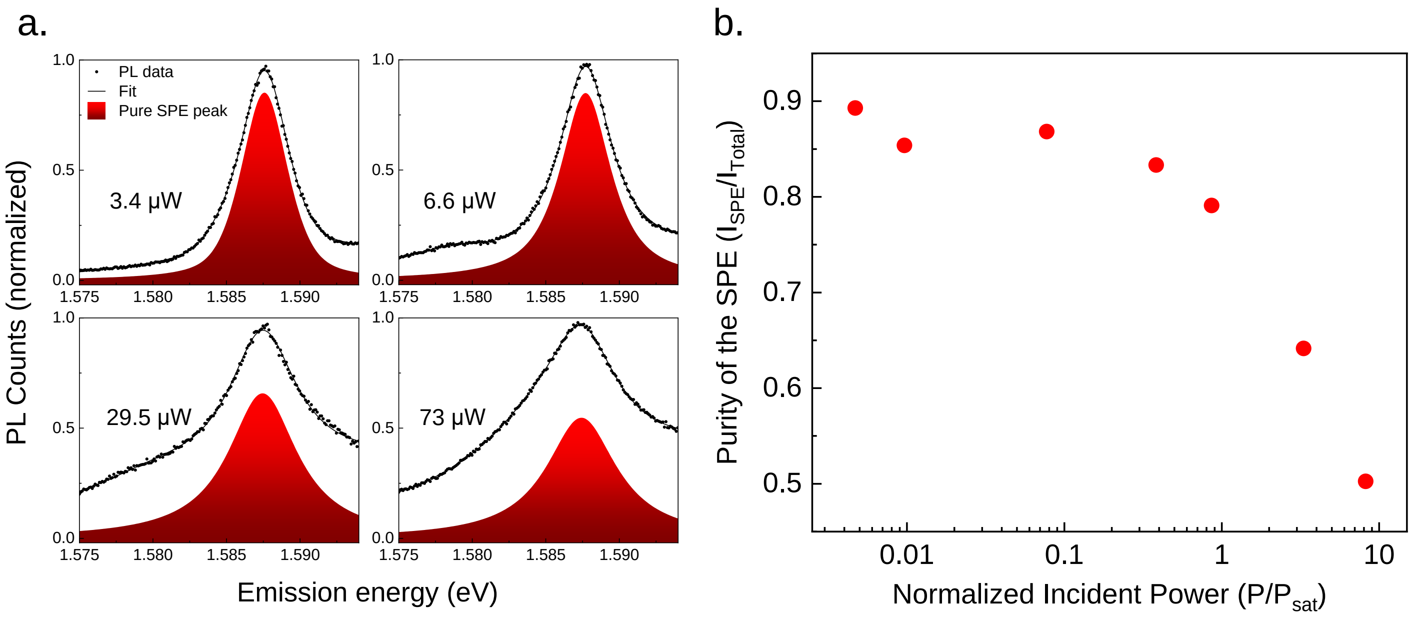


Supporting Figure 2: **variation of SPE purity with incident power. a** PL spectra from one of the pillars taken at four different incident power values. Measured PL data in black symbols, the black trace is fit to the data, and the shaded red peak is the fitted SPE peak after the removal of the contribution from the side peaks and background. **b** Ratio of the SPE intensity and the total intensity (integrated up to the FWHM). The ratio directly correlates with the purity of the photons collected by the SPAD.

Figure 2a shows the rise in the non-SPE emission with increasing incident power for one of the nanopillars. Since the SPE has a strong saturating behavior and the background emission does not, the gap between the total and pure SPE emissions widens as the incident power increases. PL counts for this device are integrated within its FWHM for both the raw PL and the fitted SPE peak (contributions from other sources removed). Since the counts measured by the SPAD correspond to the raw PL counts, we plot the ratio of SPE counts to that of SPAD

counts in Figure 2b. The rapid decrease in the purity of the counts measured by the SPAD with incident power shows that SPAD counts can erroneously inflate the emission rate such that only a fraction of the measured photons are from the SPE. Note that this data is taken from our sample with SPE peak red-shifted compared to broad defect emission of $WSe_2$ and has a gold-coated substrate, which cuts down the background emission to a good extent. Thus, this ratio can be even worse for other device designs.

# Supporting Information 4: High emission rate from more samples

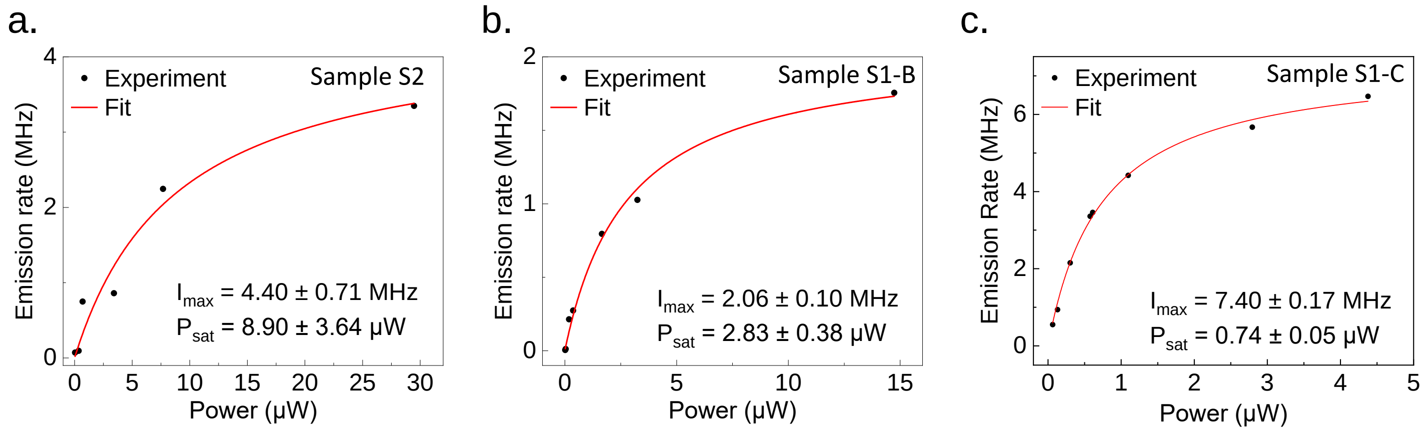


Supporting Figure 3: **Power dependent Emission rate from multiple samples. a-c** Integrated (within FWHM) emission rate measured for 3 different samples apart from the ones presented in the main text.

## Supporting Information 5: $g^{(2)}(\tau)$ from SPE shown in Figure 3c in main text

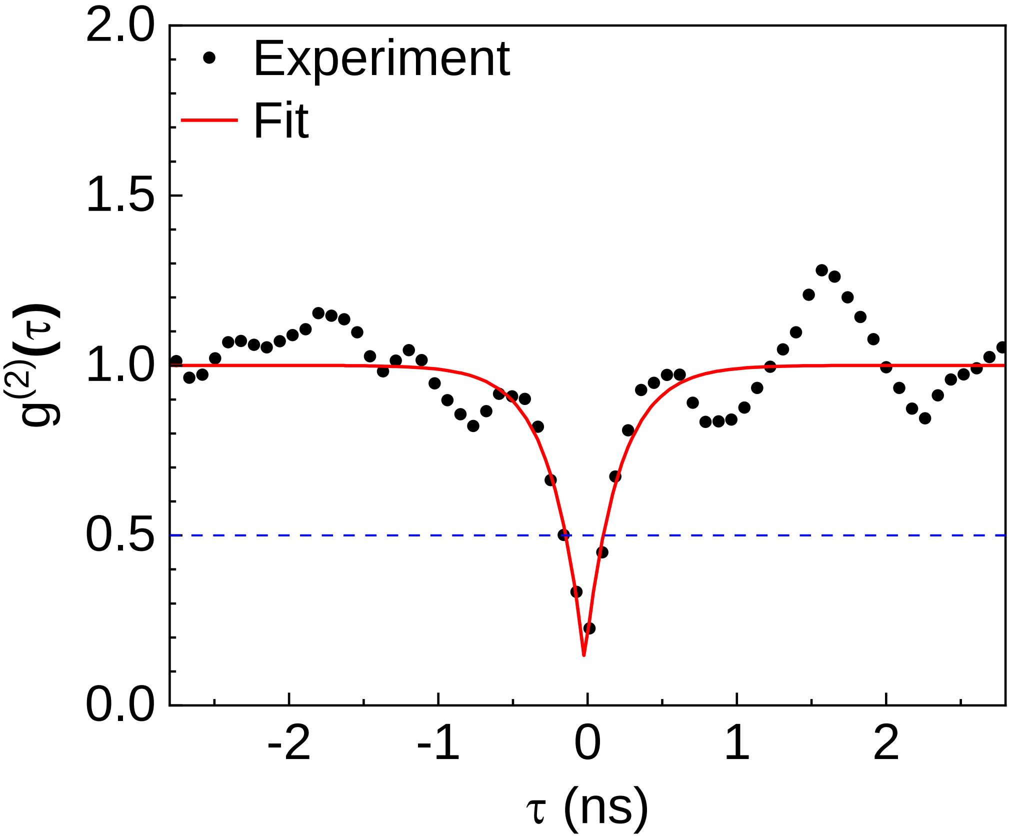


Supporting Figure 4: $g^{(2)}(\tau)$ **from SPE shown in Figure 3c in main text.** Second-order correlation measurement for the device with linewidth of 520 $\mu$eV. Experimental data in symbols, fitting in solid red trace.

## Supporting Information 6: $g^{(2)}(0)$ from a device with lower aspect ratio (sample S2)

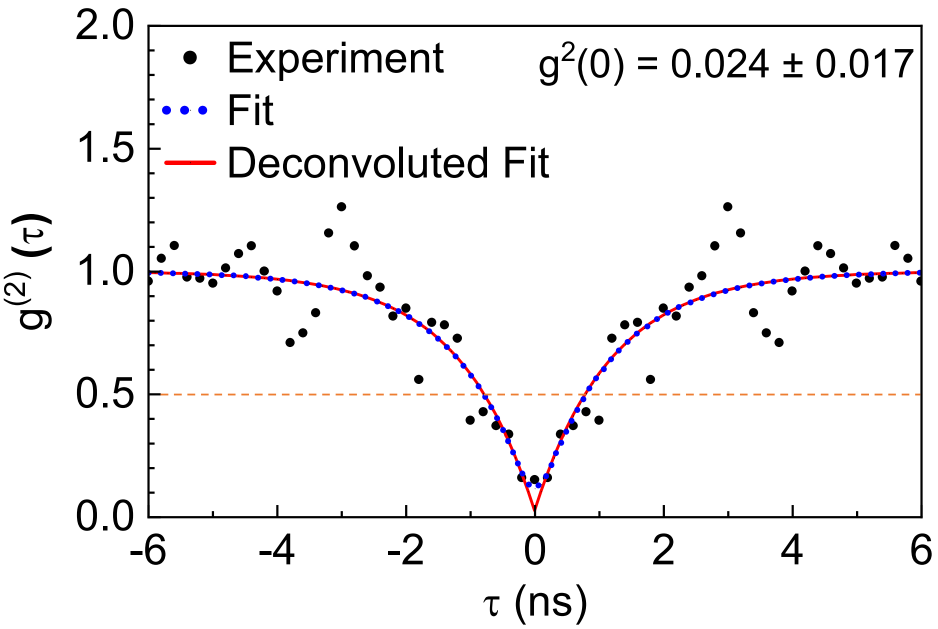


Supporting Figure 5: $g^{(2)}(\tau)$ **from a device with lower aspect ratio (sample S2).** Second-order correlation measurement for the device with lower aspect ratio of 0.27 (sample S2). Experimental data in symbols, fitting in the blue dots and deconvoluted curve in solid red trace. The $g^{(2)}(0)$ value obtained after deconvolution is $0.024 \pm 0.017$, which is well below 0.5 (indicated by dashed orange line)

## Supporting Information 7: Exciton dynamics in a strain-induced potential well

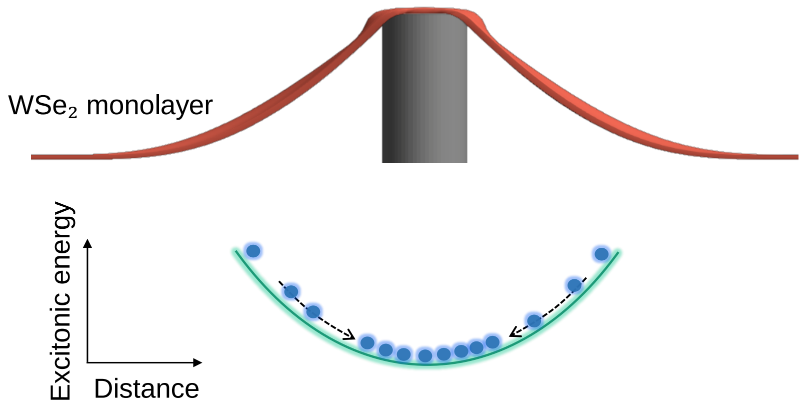


Supporting Figure 6: **Bandgap modulation and exciton dynamics under non-uniform strain** Top panel: Schematic showing a $WSe_2$ monolayer placed on a nanopillar. The TMD bends and undergoes non-uniform strain that is maximum at the center of the nanopillar. Bottom panel: Excitonic band bending due to the non-uniform strain. Excitons (blue balls) funnel to the energy minimum at the center of the nanopillar (shown by black dashed arrows).

Placing a $WSe_2$ monolayer on a nanopillar bends the monolayer introducing a non-uniform strain which is maximum on the nanopillar and gradually reduces to zero value when the flake is in contact with the substrate (See Supplementary Figure 6). The bandgap of the $WSe_2$ monolayer reduces proportional to the amount of strain applied. Thus, the bandgap minimum coincides with the center of the nanopillar in real space. Exciton band can thus be modeled as a spatially parabolic function, 2D equivalent of which is shown in Supplementary Figure 6. Excitonic energy in this parabolic band can be modeled as:

$$E_x(r) = E_{min} + \frac{1}{2}kr^2 \tag{1}$$

where $E_{min}$ is the minimum of the excitonic energy at the center of the nanopillar where the

strain is maximum, $r$ is the radial distance away from the center of the nanopillar, and $k$ correlates the gradient of excitonic band bending with the strain gradient and is proportional to the aspect ratio ($\alpha$) of the nanopillar for any particular diameter. To calibrate $k$ with $\alpha$ for the model, the strain-dependent change in excitonic energy is taken to be varying from 30.8 meV (at the center of the nanopillar) to 0 meV (at a distance of 250 nm away from the nanopillar) for an aspect ratio of 0.59. [1]

The induced electric field due to the band bending is given by:

$$E_{in}(r) = \frac{-1}{e}\frac{\partial E_x}{\partial r} \tag{2}$$

where $e$ is the electronic charge.

The total flux of the excitons in the system consists of both drift towards the center (due to the gradient in bandgap) and diffusion away from the center (due to exciton concentration gradient arising from the Gaussian generation profile of the laser) and is given by:

$$F = \mu_e n E_{in} - D_e \frac{\partial n}{\partial r} \tag{3}$$

where $\mu_e$ and $D_e$ are the mobility and diffusion coefficient of the excitons in the strain-induced potential well, respectively and n is the exciton density.

Including other exciton gain and loss mechanisms such as Gaussian generation profile of the laser [$g(r)$, a function of the excitation power P], recombination of excitons with an effective lifetime of $\tau$, and Auger annihilation (with coefficient $\gamma$), the final rate equation governing the dynamics of the excitons in the system is given by:

$$\frac{\partial n(r,t)}{\partial t} = -\frac{\partial F}{\partial r} + g(r) - \frac{n(r)}{\tau_e} - \gamma n^2(r) \tag{4}$$

At steady state ($\frac{\partial n(r,t)}{\partial t} = 0$), the equation becomes:

$$\frac{\partial F}{\partial r} = g(r) - \frac{n(r)}{\tau_e} - \gamma n^2(r) \tag{5}$$

This equation (coupled with Equation 3) was discretized by converting differentials to forward differences and was numerically solved in MATLAB to find the exciton density distribution

$[n(r)]$ as a function of $r$. Values of $\mu_e$, $D_e$, and $\gamma$ are taken from literature [2–4]. To generate the plots, we assume a nanopillar diameter of 100 nm and vary the height of the nanopillar to get different aspect ratios.

## Supporting Information 8: A generic two-level emitter

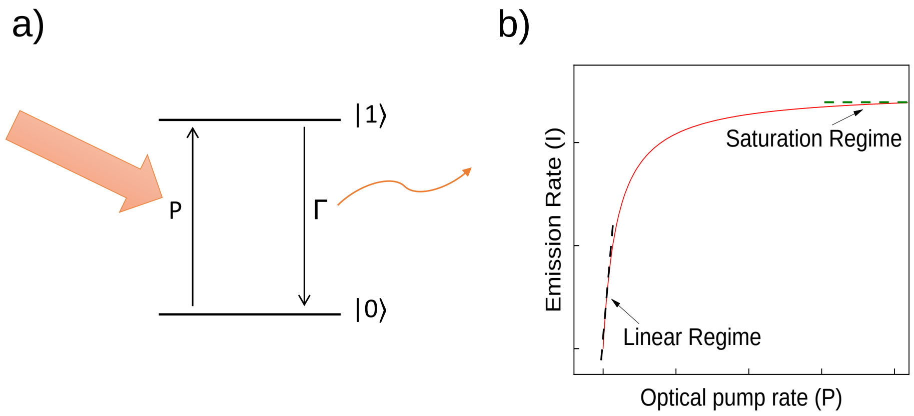


Supporting Figure 7: **A generic 2-level system.** **a** Excited state $|1\rangle$ and ground state $|0\rangle$ of a 2-level emitter with a pump rate $P$ and a recombination rate $\Gamma$. **b** Emission rate as a function of excitation power. Black dashed line shows the linear region where $P \ll \Gamma$. Green dashed line shows the saturation region where $P \gg \Gamma$.

Consider a two-level system with ground state $|0\rangle$ and excited state $|1\rangle$, as shown in Supplementary Figure 7a. The System is optically pumped from $|0\rangle$ to $|1\rangle$. The effective pumping rate is $P$ which gives a formation time for the excited state of $\tau_f = 1/P$. The system then relaxes to its ground state. Relaxation can be through radiative or non-radiative pathways. $\tau$ is the effective lifetime of the state $|1\rangle$, taking both pathways into account. The effective relaxation rate for the system is then $\Gamma = 1/\tau$. Considering $\rho_1$ and $\rho_0$ to be the occupation probabilities of the excited state and ground state, respectively, the coupled rate equations for the system can be written as:

$$\frac{d\rho_1}{dt} = \rho_0\, P - \rho_1\Gamma \tag{6}$$

$$\frac{d\rho_0}{dt} = \rho_1\, \Gamma - \rho_0 P \tag{7}$$

Since these two states are the only possible states of the system, $\rho_1 + \rho_0 = 1$. Using this

relation and considering steady state, the pair of equations (6) and (7) can be solved to get:

$$\rho_1 = \frac{P}{P + \Gamma} \tag{8}$$

Steady state emission rate of a two-level system is directly proportional to occupation probability of its excited state, therefore:

$$I \propto \frac{P}{P + \Gamma} \implies I = I_{max}\left(\frac{P}{P + \Gamma}\right) \tag{9}$$

Where $I_{max}$ is the maximum emission rate of the system, limited by its lifetime. When $P \ll \Gamma$, such that $P + \Gamma \approx \Gamma$, we have $I \approx (I_{max}/\Gamma)P$ resulting in linearity in emission vs excitation power plot (black dashed line in Supplementary Figure 7b) for small values of $P$. After increasing the excitation power much further, we reach a limit where $P \gg \Gamma$, such that $P + \Gamma \approx P$. At this point, $I \approx I_{max}$, and we see a saturation behavior in the intensity versus excitation power plot (green dashed line in Supplementary Figure 7b).

## Supporting Information 9: A Defect-based SPE coupled with an exciton reservoir

The rate of the exciton capture depends on the capture probability of individual exciton and $N_x$. Once the defect state is empty, another exciton from the excitonic band can be captured, and the process continues. If the supply of excitons in the reservoir is maintained, it emits a stream of single photons. We consider an occupation probability $\rho_d$ of the defect state such that $0 \leq \rho_d \leq 1$. Trapping of exciton from the excitonic band into the defect can be modeled as the filling of this defect state via the exciton reservoir. The rate of this filling is $(1-\rho_d)N_x\Gamma_{trap}$, where $N_x$ is the exciton reservoir population i.e. the total exciton population near the defect within its capture cross-section, $\Gamma_{trap}$ is the rate of exciton trapping, and $(1-\rho_d)$ is the probability of the defect state being unoccupied. This term ensures that the probability of capture of another exciton when the defect is already occupied is zero. Similarly, the rate of emptying of the defect state is $\rho_d\Gamma_d$, where $\Gamma_d$ is the electron-hole recombination rate through both radiative and non-radiative pathways and is inverse of the effective lifetime $\tau_d$ of the defect state.

Combining both of these factors, the rate equation for our SPE two-level system is given by:

$$\frac{d\rho_d}{dt} = (1-\rho_d)N_x\Gamma_{trap} - \rho_d\Gamma_d \tag{10}$$

At steady state $\frac{d\rho_d}{dt} = 0$ which results in the following solution:

$$\rho_d = \frac{N_x\Gamma_{trap}}{N_x\Gamma_{trap} + \Gamma_d} \tag{11}$$

Emission rate of the system is proportional to both the occupation probability $(\rho_d)$ of its excited state and the radiative decay rate of the excited state $(\Gamma_{dr})$. Thus it is given by:

$$I_{SPE} = \Gamma_{dr}\left(\frac{N_x\Gamma_{trap}}{N_x\Gamma_{trap} + \Gamma_d}\right) \tag{12}$$

Thus, the maximum achievable rate for the SPE is the radiative lifetime limited rate of $\Gamma_{dr}$.

Note that the term $N_x\Gamma_{trap}$ in Equation 12 is analogous to the Pump rate term $P$ in

Equation 9. Therefore, the formation time here can be approximated as $\tau_f \approx \frac{1}{N_x \Gamma_{trap}}$. An important distinction between the two is that this term can not be increased to an arbitrary value by increasing the optical excitation power. This is because of the saturation of $N_x$, as demonstrated in subsystem 1 of the model. Therefore the condition of $N_x \Gamma_{trap} \gg \Gamma_d$ (analogous to $P \gg \Gamma$ in Supporting Information 5) is often difficult to achieve.

## Supporting Information 10: Comparison of devices with higher and lower Auger coefficients

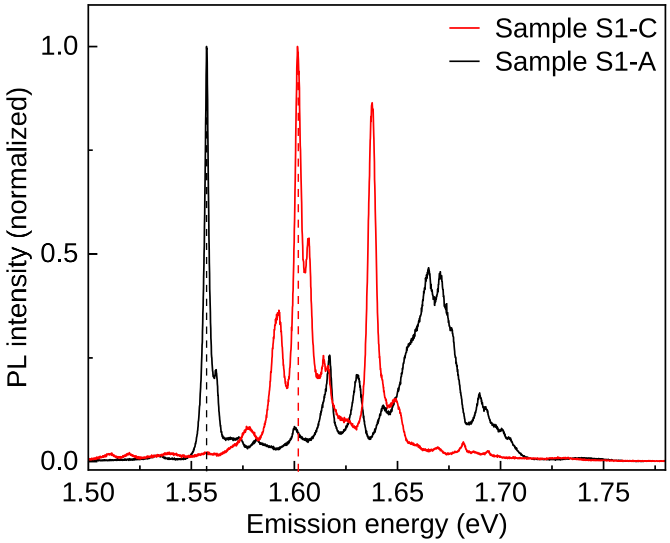


Supporting Figure 8: **Comparison of devices with higher and lower Auger coefficients.** Suppression of background defect emission analyzed through PL emission for the device fabricated with a different batch of $WSe_2$ (sample S1-C, in red) when compared to the device presented in the main text (sample S1-A, in black).

## References


[1] Artur Branny, Santosh Kumar, Raphaël Proux, and Brian D Gerardot. Deterministic strain-induced arrays of quantum emitters in a two-dimensional semiconductor. Nature Communications, 8(1):15053, May 2017.

[2] F. Cadiz, C. Robert, E. Courtade, M. Manca, L. Martinelli, T. Taniguchi, K. Watanabe, T. Amand, A. C. H. Rowe, D. Paget, B. Urbaszek, and X. Marie. Exciton diffusion in $WSe_2$ monolayers embedded in a van der Waals heterostructure. Applied Physics Letters, 112(15):152106, April 2018.

[3] Florian Dirnberger, Jonas D. Ziegler, Paulo E. Faria Junior, Rezlind Bushati, Takashi Taniguchi, Kenji Watanabe, Jaroslav Fabian, Dominique Bougeard, Alexey Chernikov, and Vinod M. Menon. Quasi-1D exciton channels in strain-engineered 2D materials. Science Advances, 7(44):eabj3066, October 2021.

[4] Long Yuan and Libai Huang. Exciton dynamics and annihilation in $WS_2$ 2D semiconductors. Nanoscale, 7(16):7402, 2015.
